# Supplementary material for: Data Drift Monitoring for Log Anomaly Detection Pipelines
Source: arXiv:2310.14893 source file (2023-10-17)
Supplement: Supplementary file 1 [file supplement.tex]

% If your paper is accepted, change the options for the package
% aistats2022 as follows:
%
%\usepackage[accepted]{aistats2024}
%
% This option will print headings for the title of your paper and
% headings for the authors names, plus a copyright note at the end of
% the first column of the first page.

% If you set papersize explicitly, activate the following three lines:
%\special{papersize = 8.5in, 11in}
%\setlength{\pdfpageheight}{11in}
%\setlength{\pdfpagewidth}{8.5in}

% If you use natbib package, activate the following three lines:
%\usepackage[round]{natbib}
%\renewcommand{\bibname}{References}
%\renewcommand{\bibsection}{\subsubsection*{\bibname}}

% If you use BibTeX in apalike style, activate the following line:
%\bibliographystyle{apalike}

%\begin{document}

% If your paper is accepted and the title of your paper is very long,
% the style will print as headings an error message. Use the following
% command to supply a shorter title of your paper so that it can be
% used as headings.
%
%\runningtitle{I use this title instead because the last one was very long}

% If your paper is accepted and the number of authors is large, the
% style will print as headings an error message. Use the following
% command to supply a shorter version of the authors names so that
% they can be used as headings (for example, use only the surnames)
%
%\runningauthor{Surname 1, Surname 2, Surname 3, ...., Surname n}

% Supplementary material: To improve readability, you must use a single-column format for the supplementary material.
\onecolumn
\aistatstitle{
Supplementary Materials}

\section{Algorithm definitions
\label{ssec:sub_algorithms}}

Vector-valued objects are denoted in bold, like $\boldsymbol{X}$, with length $|\bolsymbol{X}|$ and 1-indexing.  $E(\boldsymbol{X})$ represents the result of dividing a positive-valued vector $\boldsymbol{X}$ elementwise by the sum of element values (i.e., converting its elements to probabilities).   $X=\{a,b\}$ denotes an ordered sequence (1-indexed) of elements $a$ and $b$.  Depending on context, $X[i]$ and $\boldsymbol{X}[i]$ indicate the $\nth{i}$ element of the list or vector; similarly, $X[i:]$ and $\boldsymbol{X}[i:]$ mean the list or vector beginning with the $\nth{i}$ element, dropping the first $i-1$.

\begin{algorithm}
    %\hline
    \caption{Gamma constant in multinomial log-likelihood (see \cite{lindon2022multinomial}, Equation 27)\label{alg:multinomial_loglike}}
    \begin{algorithmic}[1]
    \Procedure{LG}{
        $X$}
        \State \Return \sum_{i=1}^{|\boldsymbol{W}|}\ln{(\Gamma(\boldsymbol{W}[i]))} - \ln{(\sum_{i=1}^{|\boldsymbol{W}|}\Gamma(\boldsymbol{W}[i]))}
    
    \end{algorithmic}
\end{algorithm}

\begin{algorithm}
    %\hline
    \caption{Windowed BF algorithm \label{alg:windowed_bf}}
    \begin{algorithmic}[1]
    \Procedure{WindowedBF}{
        $\prior{\boldsymbol{\alpha}}{}, C=\{\boldsymbol{C}_1,\boldsymbol{C}_2,\dots\},\kappa,w,B_0=0$}
        \LineComment{$\prior{\boldsymbol{\alpha}}{}$: Prior multinomial vector of non-drifted logs}
        \LineComment{$\boldsymbol{C}$: sequence of observed count vectors}
        \LineComment{$\kappa$: positive constant to rescale count vectors by}
        \LineComment{$w$: integer, $w\geq 2$ window size to use in drift detection}
        \LineComment{$B_0$: log prior odds on log-BF}
        \State $W\gets \{\boldsymbol{0}\}$ \Comment{Window of count vectors to keep}
        \State $W_S\gets \{\prior{\boldsymbol{\alpha}}{}\}$ \Comment{Cumulative sums of $W$}
        \State $B\gets \{\}$ \Comment{log-BF sequence}
        \State $\boldsymbol{\theta}_0 \gets E(\prior{\boldsymbol{\alpha}}{})$
        %\While{$t< |C|$}
        \For{$t=1\textrm{ \textbf{to} }|C|$}
            \State $\tilde{\boldsymbol{C}}_t\gets \kappa \times E(\boldsymbol{C}_t)$
        \If{$t>w$}
            \IndentLineComment{Drop element outside of window $w$}
            \State $W \gets W[\:2:\:]$
        \EndIf
        \For{$i=2\textrm{ \textbf{to} }|W_S|$} 
            \LineComment{Window-constrained cumulative estimate of $\post{\boldsymbol{\alpha}}{i}$}
            \State $W_S[i] \gets W_S[i-1] + W[i-1]$
        \EndFor
        \LineComment{Apply recursive formula Algorithm~\ref{alg:multinomial_loglike} for log-BF at $t$ in current window $W$}
        \State $B[t]\gets B_0+\sum_{i=1}^{|W|}\left(LG({W}_S[i] + W[i]) - LG(W_S[i])-\sum_{j=1}^{|\boldsymbol{C}_t|}\ln{(W[i][j])}\boldsymbol{\theta_0}[j]\right)$
        \LineComment{Append newest count vector to window}
        \State $W[\:|W|+1\:]\gets \tilde{\boldsymbol{C}}_t$
    \EndFor
    \State \Return $B$
    \end{algorithmic}
\end{algorithm}
